# Supplementary material for: Isekai3D SDG: A Platform for Diverse Synthetic Gameplay Visual Data
Source: arXiv:2611.03626 source file (2026-11-02)
Supplement: Supplementary file 1 [file 0_main.tex]

\section{Appendix}
